# Supplementary material for: Effects of thermal, elastic, and surface properties on the stability of SiC polytypes
Source: arXiv:2201.05379 source file (2022-08-15)
Supplement: Supplementary file 1 [file SM_ramakers_resubmission2_final.pdf]

# SM: Effects of thermal, elastic and surface properties on the stability of SiC polytypes

Senja Ramakers,[1,2,*] Anika Marusczyk,[1] Maximilian Amsler,[1] Thomas Eckl,[1] Matous Mrovec,[2] Thomas Hammerschmidt,[2] and Ralf Drautz[2]

[1]*Corporate Sector Research and Advance Engineering, Robert Bosch GmbH, Robert-Bosch-Campus 1, 71272 Renningen, Germany*

[2]*Interdisciplinary Centre for Advanced Materials Simulation, Ruhr-Universität Bochum, Universitätsstraße 150, 44801 Bochum Germany*

(Dated: August 12, 2022)

## I. POLYTYPE STABILITY REPORTED IN THE LITERATURE

TABLE I. Overview of literature reporting on the polytype stability, references are sorted from oldest to newest. TM means Troullier-Martin, BHS means Bachelet-Hamann-Schaetle, LAPW means Linearized Augmented Planewave method, PAW means Projector Augmented Wave method.

| Reference | Method | Pseudopotential | $\Delta E_{2H}$ | $\Delta E_{4H}$ | $\Delta E_{6H}$ |
|---|---|---|---|---|---|
| Cheng et al.[1] | DFT-LDA | Norm conserving | 9.9 | -1.9 | - |
| Park et al.[2] | DFT-LDA | TM[3] | 4.0 | -4.6 | -3.0 |
| Kaeckell et al.[4] | DFT-LDA[5] | BHS[6] | 1.8 | -3.8 | -3.0 |
| Karch et al.[7] | DFT-LDA-PZ[8] | TM[3] | 4.9 | -2.7 | - |
| Limpijumnong et al.[9] | LDA-GGA-PW91[10] | All electron | 5.4 | -2.4 | -1.1 |
| Jiang et al.[11] | DFT-LDA | Vanderbilt[12] | 4.0 | -2.4 | -2.9 |
| | DFT-LDA | Lin[13] | 5.2 | -2.5 | -2.8 |
| Bernstein et al.[14] | DFT-LDA-PW91[10] | LAPW[15,16] | 4.6 | -4.2 | -3.2 |
| Konstantinova et al.[17] | DFT-LDA | TM[3] | - | -3.6 | -3.2 |
| Ito et al.[18] | DFT-GGA | TM[3] | 11.4 | 0.04 | 0.5 |
| Mercier et al.[19] | DFT-GGA-PW91[10] | Ultrasoft | 5.8 | -0.2 | -0.4 |
| Ito et al.[20] | ANNNI model[21] | - | 11.0 | 0.5 | 0.4 |
| Kawanishi et al.[22] | DFT-LDA[5] | PAW[23,24] | 4.4 | -3.0 | -2.6 |
| | DFT-GGA-PBE[25] | PAW[23,24] | 5.8 | -1.5 | -1.4 |
| | DFT-GGA-PBE[25] +vdW-D2[26] | PAW[23,24] | 14.8 | 2.4 | 1.2 |

## II. NUMERICAL CONVERGENCE

The numerical convergence of the plane wave cut-off energy and k-mesh is shown in Fig. 1. We chose the value of the k-mesh around 4096 k-points per reciprocal atom (KPPRA), see Table I for the exact values per unit cell for each polytype. The cut-off energy converges to $<1$ meV/SiC at 1000 eV and to $<0.1$ meV/SiC at 1500 eV. The latter stringent criterium was required to get smooth curves for the differences of the energy-strain curves between the polytypes, as described in Section III D.

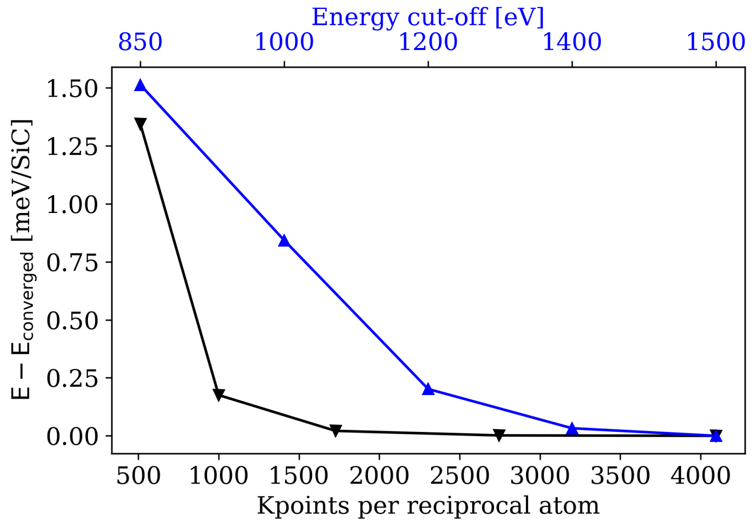


FIG. 1. K-mesh and cut-off energy convergence for an eight atom cubic 3C-SiC cell.

## III. INTERNAL ENERGY DIFFERENCES BETWEEN 3C AND THE $x$H POLYTYPES

TABLE II. Results of the internal energies at $T = 0$ K shown in Fig. 1 (non-vdW methods) and Fig. 2 (vdW methods).

| Method | $\Delta E_{6\text{H}}$ 33% | $\Delta E_{4\text{H}}$ 50% | $\Delta E_{2\text{H}}$ 100% |
|---|---|---|---|
| VASP LDA | -2.16 | -2.46 | 4.71 |
| VASP PW91 | -1.17 | -1.02 | 6.40 |
| VASP PBE | -1.36 | -1.33 | 5.86 |
| VASP PBEsol | -2.41 | -2.79 | 4.04 |
| VAPS HSE06 | -1.31 | -1.47 | 4.72 |
| VASP SCAN | -0.01 | 0.50 | 8.99 |
| VASP RTPSS | -2.20 | -2.41 | 7.48 |
| CP2K PBE DZVP-SR | -1.13 | -0.71 | 8.24 |
| CP2K PBE TZV2PX | -1.56 | -1.84 | 4.53 |
| CP2K PBE NLCC TZV2PX | -1.50 | -1.72 | 4.82 |
| FHI-aims PBE tight | -1.89 | -1.99 | 4.36 |
| FHI-aims PBE really tight | -1.68 | -1.65 | 4.89 |
| VASP PBE-D2 | 1.60 | 3.15 | 14.94 |
| VASP PBE-D3 | -0.97 | -0.73 | 7.25 |
| VASP PBE-D3/BJ | -1.14 | -0.97 | 12.34 |
| VASP PBE-TS | -3.29 | -4.23 | 0.45 |
| VASP PBE-TS/HI | -1.54 | -1.54 | 5.92 |
| VASP PBE-MBD | -1.59 | -1.34 | 6.87 |
| VASP vdW-DF2 | 0.65 | 1.61 | 11.23 |
| VASP optPBE-vdW | 1.01 | 2.07 | 11.59 |
| VASP optB88-vdW | 1.55 | 2.50 | 12.34 |

## IV. EFFECT OF THE LATTICE ON THE POLYTYPES' ENERGY DIFFERENCES

In Figs. 2 and 5, we show the relative energies between 3C and the $x$H polytypes for the various computational methods. The results were obtained for the relaxed lattice parameters of each method, which vary around the experimental value as visible in Figs. 3 and 4. To understand the effect of the lattice parameter on the energy differences between the polytypes, we compare these results to the energy differences calculated for the fixed experimental lattice parameters[27,28]. We performed the calculations with five representative computational methods (local, semilocal, one vdW correction, and one meta-GGA).

Overall, fixing the lattice parameter to the experimental value does not change the results significantly. For 4H and 6H, the spread is $<10\%$ of the total energy difference to 3C (between 0.03 and 0.27 meV/SiC). Methods which predict lattice parameters that deviate more from the experimental values show a wider spread in energy. This can be understood by the fact that when the deviation is greater, you move away from the equilibrium on the energy-strain curve (Fig. 8), which will result in a different relative energy. The maximum difference is $E_{3C}$-$E_{2H}$ $= -0.97$ meV (-20%) for 2H calculated with LDA. Fig. 3 shows that LDA is an outlier regarding the predicted lattice parameters. Thus, the accuracy of the predicted lattice parameter is directly related to the spread in energy. However, the wide variety in energies between the different methods from Figs. 2 and 3 is just as apparent with the fixed as with the relaxed lattice. We conclude that the spread in relative energies between the different methods is not an artefact of differing relaxed lattice parameters but rather caused by the computational methods themselves.

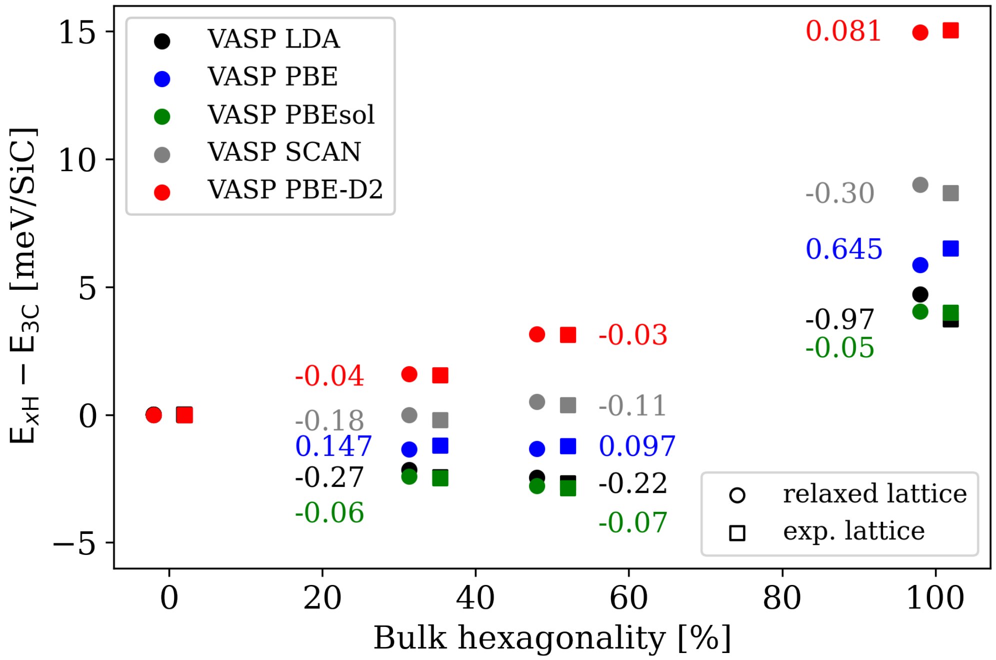


FIG. 2. Relative energies of the polytypes for relaxed and fixed experimental lattice from Ref. 27 (3C, 4H, 6H) and Ref. 28 (2H). For visualization, the datapoints are slightly moved to the left (relaxed) and right (experimental) from the ideal hexagonality. The numbers show the energy differences between relaxed and fixed lattice parameter in meV/SiC.

## V. LATTICE PARAMETERS OF 3C AND THE $x$H POLYTYPES

TABLE III. Results of the lattice parameter at $T$ = 0 K used for Fig. 3 ($a$ lattice) and Fig. 4 ($a/(2xc)$ lattice ratio).

| Method | $a_{3C}$ | $a_{6H}$ | $c_{6H}$ | $a_{4H}$ | $c_{4H}$ | $a_{2H}$ | $c_{2H}$ |
|---|---|---|---|---|---|---|---|
| exp. Levinshtein et al. | 4.3596 | 3.0805 | 15.1151 | 3.0798 | 10.0820 | - | - |
| exp. Stockmeier et al. | - | 3.08049 | 15.11507 | 3.07976 | 10.08196 | - | - |
| exp. Harris et al. | - | 3.08049 | 15.11507 | 3.07976 | 10.08196 | - | - |
| VASP LDA | 4.3314 | 3.0610 | 15.0200 | 3.0601 | 10.0183 | 3.0580 | 5.0190 |
| VASP PW91 | 4.3795 | 3.0946 | 15.1847 | 3.0939 | 10.1285 | 3.0914 | 5.0737 |
| VASP PBE | 4.3805 | 3.0955 | 15.1895 | 3.0947 | 10.1311 | 3.0924 | 5.0752 |
| VASP PBEsol | 4.3587 | 3.0804 | 15.1143 | 3.0796 | 10.0811 | 3.0773 | 5.0502 |
| CP2K PBE DZVP-SR | 4.3730 | 3.0900 | 15.1677 | 3.0889 | 10.1193 | 3.0866 | 5.0708 |
| CP2K PBE TZV2PX | 4.3690 | 3.0875 | 15.1494 | 3.0867 | 10.1049 | 3.0846 | 5.0619 |
| CP2K PBE NLCC TZV2PX | 4.3804 | 3.0955 | 15.1905 | 3.0946 | 10.1324 | 3.0924 | 5.0765 |
| FHI-aims PBE t & rt | 4.3805 | 3.0955 | 15.1895 | 3.0947 | 10.1311 | 3.0924 | 5.0752 |
| VASP SCAN | 4.3503 | 3.0743 | 15.0859 | 3.0731 | 10.0614 | 3.0710 | 5.0422 |
| VASP RTPSS | 4.3606 | 3.0818 | 15.1241 | 3.0805 | 10.0876 | 3.0787 | 5.0544 |
| VASP PBE-D2 | 4.3555 | 3.0777 | 15.1162 | 3.0767 | 10.0871 | 3.0739 | 5.0592 |
| VASP PBE-D3 | 4.3672 | 3.0862 | 15.1423 | 3.0854 | 10.0991 | 3.0832 | 5.0578 |
| VASP PBE-D3/BJ | 4.3494 | 3.0736 | 15.0813 | 3.0729 | 10.0595 | 3.0706 | 5.0392 |
| VASP PBE-TS | 4.3606 | 3.0815 | 15.1040 | 3.0805 | 10.0694 | 3.0781 | 5.0340 |
| VASP PBE-TS/HI | 4.3573 | 3.0793 | 15.1097 | 3.0785 | 10.0784 | 3.0762 | 5.0494 |
| VASP PBE-MBD | 4.3547 | 3.0774 | 15.1004 | 3.0766 | 10.0722 | 3.0742 | 5.0461 |
| VASP vdW-DF2 | 4.3803 | 3.0953 | 15.1884 | 3.0944 | 10.1305 | 3.0922 | 5.0750 |
| VASP optPBE-vdW | 4.3910 | 3.1022 | 15.2274 | 3.1012 | 10.1577 | 3.0986 | 5.0897 |
| VASP optB88-vdW | 4.3773 | 3.0942 | 15.1859 | 3.0924 | 10.1280 | 3.0904 | 5.0751 |

## VI. VAN DER WAALS METHODS

In this Section, we give a brief description of the van der Waals methods employed in our work. For more extensive information we recommend the review article of Hermann et al.[29].

First, we discuss pairwise interaction correction methods, which do not consider many-body effects. The DFT-D2 method[26] applies a correction term to the total energy calculated with a conventional DFT method, in our case VASP-PBE. The correction is calculated by evaluating the pairwise interaction of atoms with a suitable distance. A damping function minimizes the contributions from interaction within typical bonding distances, and atom pairs with a distance $> 50$ Å are disregarded. Only the 6th-order dispersion coefficients are considered. The coefficients are fixed per element and fitted to experimental data. Thus, they are empirical and insensitive to the local chemical environment. The improved version DFT-D3 was introduced some years later[30]. The main changes are that also the 8th-order dispersion coefficients is included, and that the coefficients are geometry dependent. Together with some smaller modifications, this decreases the error by 15%-40% compared to the earlier method. Although the damping has only a minor impact on the correction[30], efforts have been made to describe the asymptotic behavior more correctly. Becke and Johnson introduced a new damping function that was implemented as DFT-D3/BJ[30,31].

The Tkatchenko-Scheffler method, vdW-TS, was introduced to overcome the empirical nature of other pairwise methods like DFT-D[32]. This method includes the 6th-order dispersion. However, the dispersion coefficient and damping are determined by incorporating information of the local chemical environment via the electron density. The method is known to describe ionic solids rather inaccurately. The vdW-TS/HI method[33,34] aims to improve this behavior by employing an iterative Hirschfeld (HI) partitioning algorithm[35].

The last vdW correction method evaluated in this work is the vdW-MBD method[36,37]. It goes beyond pairwise interaction and introduces Many-Body Dispersion effects. The dispersion energy is based on the random phase approximation (RPA) for the correlation energy. Here, the long-range many-body vdW energy is obtained from the solution of the Schroedinger equation for a system of coupled oscillators[32]. The method's formalism is mathematically equivalent to RPA. Nonetheless, the method still employs the same scheme as the vdW-TS, where the coefficients are derived by scaling reference data of the free atomic values.

The previously discussed methods all employ a correction term added to the conventional DFT total energy. Another way to incorporate vdW dispersion is directly through the XC functional. The vdW-DF functionals[38–40] evaluate the correlation energy in two separate non-local approximations. The first approximation accounts for the local correlation through the regular LDA correlation energy. The second term is a full electronic potential approximation, which determines the long-range interactions. The exchange energy is calculated with GGA, of which there are several functionals available. In this work, we review the original vdW-DF2 functional and the PBE (optPBE-vdW) and B88 (optB88-vdW) versions[41,42].

## VII. (0001) AND (000$\bar{1}$) SURFACE ENERGIES OF 3C-SIC AND THE $x$H-SIC

TABLE IV. Results of the surface energies used for Figs. 10 and 11 in J/m$^2$.

| Type | 3C | 6H-S3 | 6H-S2 | 4H-S2 | 6H-S1 | 4H-S1 | 2H |
|---|---|---|---|---|---|---|---|
| Si-terminated (0001), non-spin-polarized | 2.731 | 2.777 | 2.805 | 2.819 | 2.903 | 2.924 | 2.982 |
| Si-terminated (0001), $(2 \times 1)$ reconstructed | 2.550 | 2.584 | 2.601 | 2.612 | 2.656 | 2.671 | 2.715 |
| Si-terminated (0001), ferromagnetic | 2.407 | 2.429 | 2.430 | 2.442 | 2.483 | 2.488 | 2.507 |
| C-terminated (000$\bar{1}$), non-spin-polarized | 3.878 | 3.902 | 3.897 | 3.908 | 3.806 | 3.815 | 3.828 |
| C-terminated (000$\bar{1}$), ferromagnetic | 3.410 | 3.425 | 3.417 | 3.429 | 3.436 | 3.438 | 3.436 |

* senja.ramakers@de.bosch.com

[1] C. Cheng, Europhysics Letters (1987).

[2] C. H. Park, B.-H. Cheong, K.-H. Lee, and K. J. Chang, Physical Review B **49**, 4485 (1994).

[3] N. Troullier and J. L. Martins, Physical Review B **43**, 1993 (1991).

[4] P. Käckell, B. Wenzien, and F. Bechstedt, Physical Review B **50**, 10761 (1994).

[5] D. M. Ceperley and B. J. Alder, Physical Review Letters **45**, 566 (1980).

[6] G. B. Bachelet, D. R. Hamann, and M. Schlüter, Physical Review B **26**, 4199 (1982).

[7] K. Karch, P. Pavone, W. Windl, O. Schütt, and D. Strauch, Physical Review B **50**, 17054 (1994).

[8] J. P. Perdew and A. Zunger, Physical Review B **23**, 5048 (1981).

[9] S. Limpijumnong and W. R. Lambrecht, Physical Review B **57**, 12017 (1998).

[10] J. P. Perdew, J. A. Chevary, S. H. Vosko, K. A. Jackson, M. R. Pederson, D. J. Singh, and C. Fiolhais, Physical Review B **46**, 6671 (1992).

[11] Z. Jiang, X. Xu, H. Wu, F. Zhang, and Z. Jin, Solid state communications **123**, 263 (2002).

[12] D. Vanderbilt, Physical Review B **41**, 7892 (1990).

[13] S.-k. Lin, C.-k. Yeh, B. Puchala, Y.-L. Lee, and D. Morgan, Computational Materials Science **73**, 41 (2013).

[14] N. Bernstein, H. J. Gotsis, D. A. Papaconstantopoulos, and M. J. Mehl, Physical Review B **71** (2005), 10.1103/PhysRevB.71.075203.

[15] O. K. Andersen, Physical Review B **12**, 3060 (1975).

[16] S.-H. Wei and H. Krakauer, Physical Review Letters **55**, 1200 (1985).

[17] E. Konstantinova, M. Bell, and V. Anjos, Intermetallics **16**, 1040 (2008).

[18] T. Ito, T. Kondo, T. Akiyama, and K. Nakamura, Journal of Crystal Growth **318**, 141 (2011).

[19] F. Mercier and S.-i. Nishizawa, Journal of Crystal Growth **360**, 189 (2012).

[20] T. Ito, T. Akiyama, and K. Nakamura, Journal of Crystal Growth **362**, 207 (2013).

[21] J. Smith, J. Yeomans, and V. Heine, in *Modulated Structure Materials*, edited by T. Tsakalakos (Springer Netherlands, Dordrecht, 1984) pp. 95–105, dOI: 10.1007/978-94-009-6195-1_5.

[22] S. Kawanishi and T. Mizoguchi, Journal of Applied Physics **119**, 175101 (2016).

[23] P. E. Blöchl, O. Jepsen, and O. K. Andersen, Physical Review B **49**, 16223 (1994).

[24] G. Kresse and D. Joubert, Physical Review B **59**, 1758 (1999).

[25] J. P. Perdew, K. Burke, and M. Ernzerhof, Physical Review Letters **77**, 3865 (1996).

[26] S. Grimme, Journal of Computational Chemistry **27**, 1787 (2006).

[27] M. E. Levinshtein, S. L. Rumyantsev, and M. S. Shur, *Properties of Advanced Semiconductor Materials: GaN, AIN, InN, BN, SiC, SiGe* (John Wiley & Sons, 2001).

[28] G. L. Harris and Institution of Electrical Engineers, eds., *Properties of silicon carbide*, EMIS datareviews series No. 13 (INSPEC, the Inst. of Electrical Engineers, London, 1995) oCLC: 263658310.

[29] J. Hermann, R. A. DiStasio, and A. Tkatchenko, Chemical Reviews **117**, 4714 (2017).

[30] S. Grimme, S. Ehrlich, and L. Goerigk, Journal of Computational Chemistry **32**, 1456 (2011).

[31] A. D. Becke and E. R. Johnson, The Journal of Chemical Physics **123**, 154101 (2005).

[32] A. Tkatchenko and M. Scheffler, Physical Review Letters **102** (2009), 10.1103/PhysRevLett.102.073005.

[33] T. Bučko, S. Lebègue, J. G. Ángyán, and J. Hafner, Journal of Chemical Theory and Computation **9**, 4293 (2013).

[34] T. Bučko, S. Lebègue, J. G. Ángyán, and J. Hafner, The Journal of Chemical Physics **141**, 034114 (2014).

[35] P. Bultinck, C. Van Alsenoy, P. W. Ayers, and R. Carbó-Dorca, The Journal of Chemical Physics **126**, 144111 (2007).

[36] A. Tkatchenko, R. A. DiStasio, R. Car, and M. Scheffler, Physical Review Letters **108** (2012), 10.1103/PhysRevLett.108.236402.

[37] A. Ambrosetti, A. M. Reilly, R. A. DiStasio, and A. Tkatchenko, The Journal of Chemical Physics **140**, 18A508 (2014).

[38] M. Dion, H. Rydberg, E. Schröder, D. C. Langreth, and B. I. Lundqvist, Physical Review Letters **92** (2004), 10.1103/PhysRevLett.92.246401.

[39] D. C. Langreth, M. Dion, H. Rydberg, E. Schröder, P. Hyldgaard, and B. I. Lundqvist, International Journal of Quantum Chemistry **101**, 599 (2005).

[40] G. Román-Pérez and J. M. Soler, Physical Review Letters **103** (2009), 10.1103/PhysRevLett.103.096102.

[41] J. Klimes, D. R. Bowler, and A. Michaelides, Journal of Physics: Condensed Matter **22**, 022201 (2010).

[42] J. Klimes, D. R. Bowler, and A. Michaelides, Physical Review B **83** (2011), 10.1103/PhysRevB.83.195131.
